# Supplementary material for: Learning Monocular 3D Human Pose Estimation from Multi-view Images
Source: arXiv:1803.04775 source file (2018-03-24)
Supplement: Supplementary file 1 [file supplemental.tex]

\begin{table*}[!b]
		\centering
\resizebox{1\linewidth}{!}{
		\begin{tabular}{ |l|c|c|c|c|c|c|c|c|c|c|c|c|c|c|c|c|c| }
			\hline
Method& Directions & Discuss & Eat & Greet & Phone & Pose & Purchase & Sit & Sitdown& Smoke & Photo & Wait & Walk & Walk Dog &  Walk Pair &  Total \\
\hline
\OURN{}
&67.0
&74.5
&77.3
&80.1
&87.8
&69.1
&73.6
&101.0
&136.0
&80.5
&100.0
&75.4
&69.1
&86.7
& 68.5
& 83.4\\
\OURW{}
&\bf 61.9
&\bf 69.4
&\bf 69.9
&\bf 75.8
&\bf 82.9
&\bf 64.3
&\bf 68.1
&\bf 91.2
&\bf 134.4
&\bf 74.2
&\bf 97.5
&\bf 70.2
&\bf 62.8
&\bf 83.4
&\bf 65.4
&\bf 78.2\\
\hline
Improvement
&5.0
&5.0
&7.4
&4.3
&5.0
&4.8
&5.5
&9.9
&1.7
&6.3 
&2.5 
&5.2 
&6.3 
&3.3
&3.1
&5.2\\
			\hline
		\end{tabular}
	}
 \vspace{1pt}
	\caption{Activity-wise NMPJPE scores in mm. As in Fig.~\ref{fig:H36Maction}, our method (\OURW) is compared to the baseline (\OURN).}
	\label{tb:H36Maction}
\end{table*}

\section{Ski Dataset}

\NEW{The capture process for the ski dataset was as follows. 
The global locations of the cameras and of static reference markers (black spheres) were geodetically measured by a tachymeter theodolite (Leica Total station 1200).
A trained annotator clicked on the visible reference markers in each view and frame to determine the camera pan, tilt and zoom. 
In the same way, 22 human joints were marked at their visual center and triangulated. 
The average Euclidean error of such procedure is $23 \pm 10$ mm, determined by comparing the photogrammetric marker estimates with the theodolite ones \cite{Klous10}.
Possible click-inaccuracies were mitigated by normalizing bone length to be constant at their anthropometrically measured values \cite{Smith94}.
Re-projection of the 3D annotation shows a very accurate overlap with the images, as visualized in the main paper. We make the dataset available to facilitate future work towards reliable monocular pose reconstruction (\href{http://cvlab.epfl.ch/Ski-PosePTZ-Dataset}{cvlab.epfl.ch/Ski-PosePTZ-Dataset}).}

\section{Action-Specific Evaluation on Human3.6M}

In the main paper, we have shown that our weakly-supervised approach based on multi-view images for training  consistently improves the accuracy of monocular human pose estimation across datasets. %
For the H36M dataset, we reported the errors averaged over all actions.
Here, by contrast, we provide the NMPJPE for each individual actions of the H36M dataset. We refer the reader to the main paper for the definition of the notation and of the baseline.
As can be seen from Table \ref{tb:H36Maction} and Fig.~\ref{fig:H36Maction}, our approach yields a consistent improvement over the baseline for all actions, with particularly high gains for the Sit (10 mm), Eat (7mm), and Walk (6 mm) classes.
This confirms the qualitative and quantitative results reported in the main paper.
\newpage
\begin{figure}
	\includegraphics[width=1\linewidth]{images/h36m/action_wise_barplot.pdf}\\
	\caption{\label{fig:H36Maction}
		{\bf Per-class accuracies on H36M.} We report the NMPJPE metric (in mm) for the baseline (\OURN, orange) and our method (\OURW, yellow) for every action of H36M. Note that our weakly-supervised scheme, leveraging multiple views during training only, consistent outperforms the baseline.}
\end{figure}
